# Supplementary material for: EasyHeC++: Fully Automatic Hand-Eye Calibration with Pretrained Image Models
Source: arXiv:2410.09293 source file (2024-10-11)
Supplement: Supplementary file 1 [file autoinit_4x4.tex]

\begin{figure}[ht]
    \centering
    \resizebox{1.0 \columnwidth}{!}{
        \includegraphics[width=0.5\linewidth]{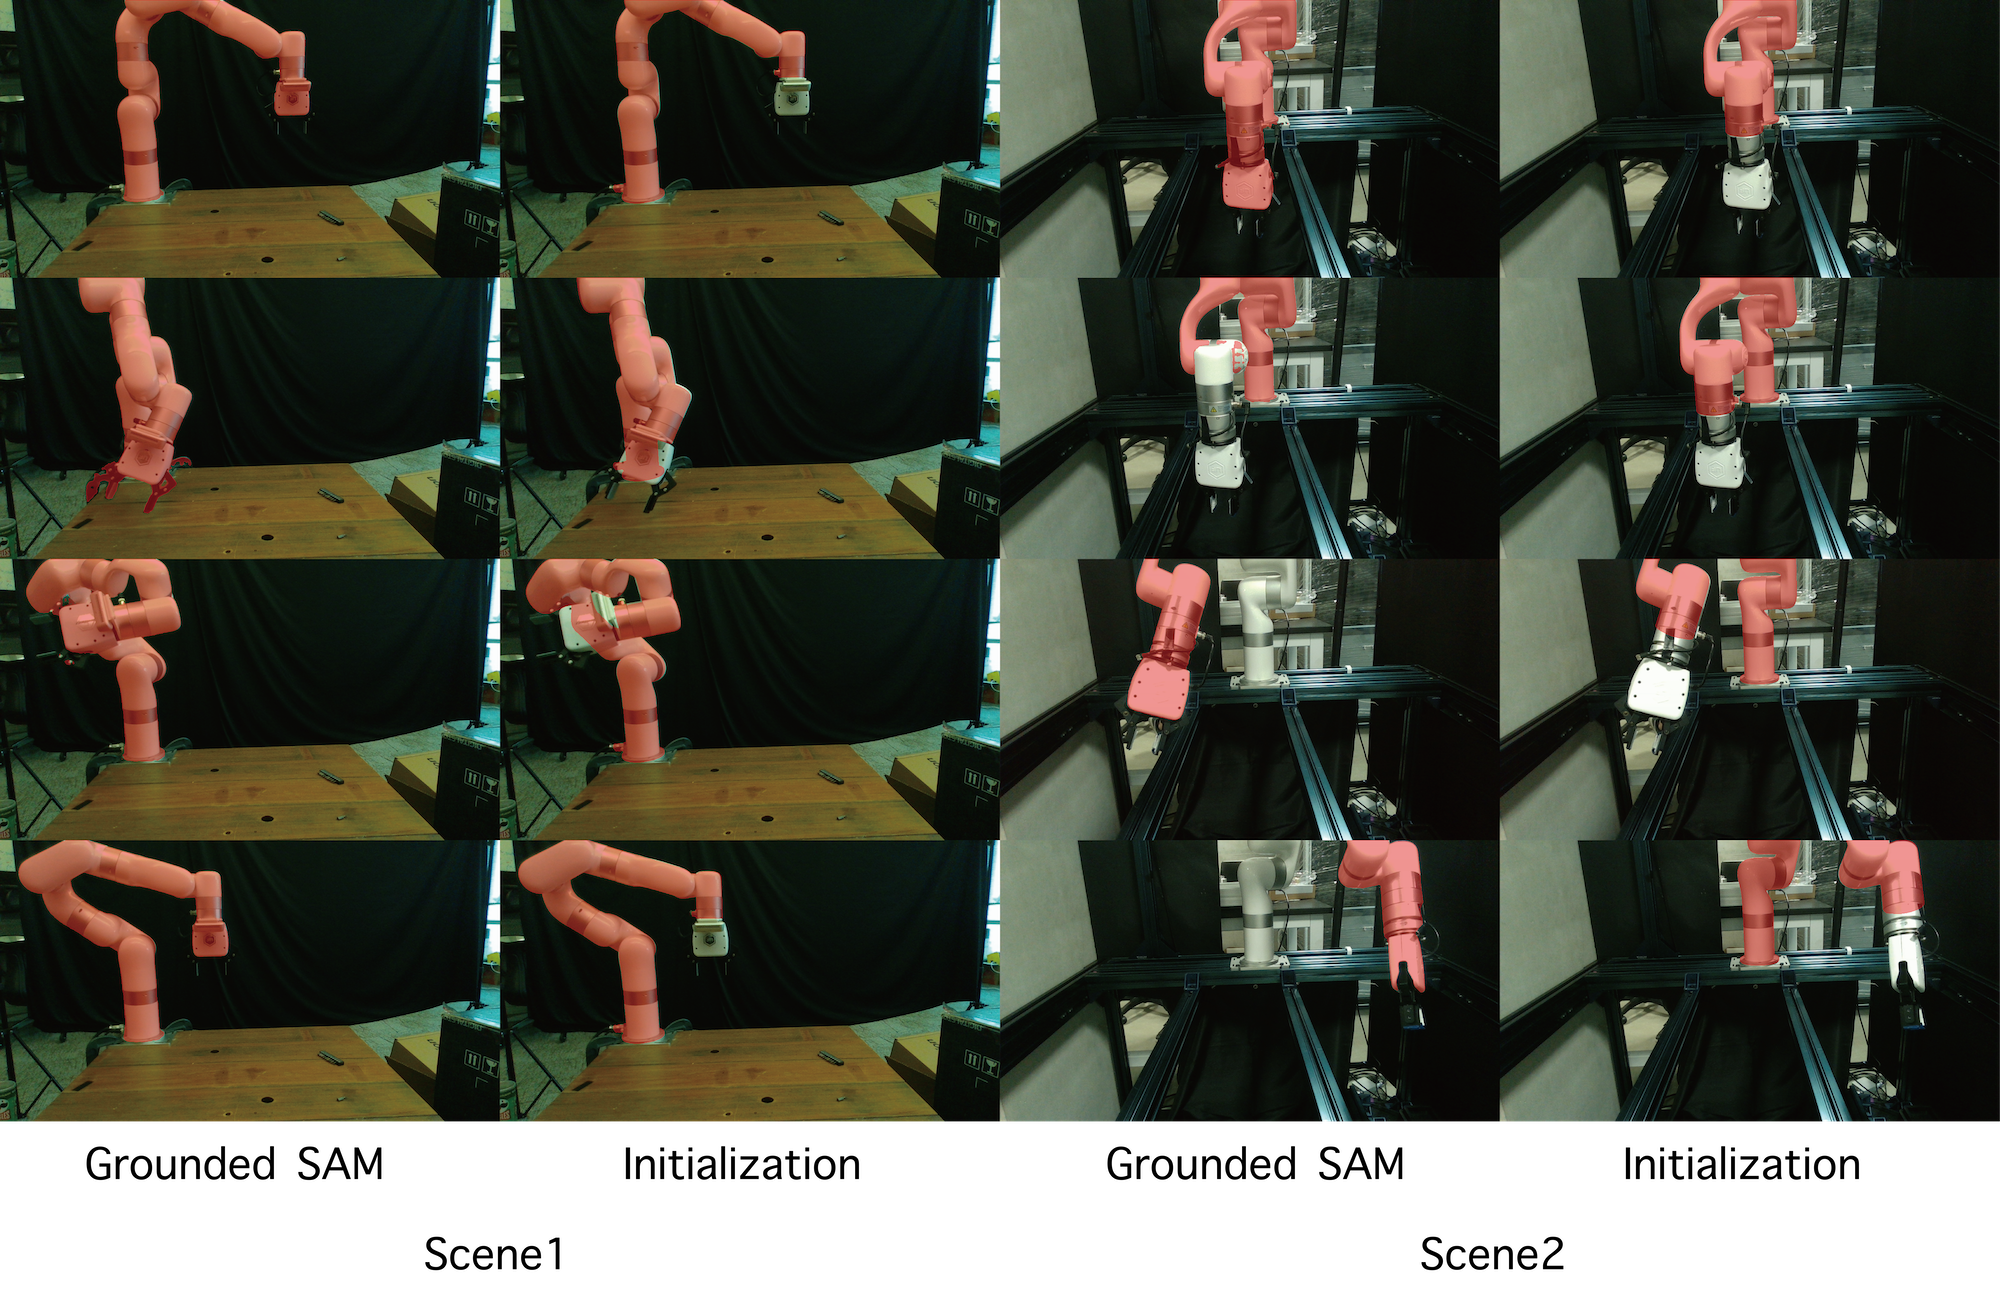}
    }
    \caption{\textbf{Example images in the sampling-based initialization process in 2 scenes.}
    We visualize the images at different joint poses and the corresponding segmentation masks predicted by the GroundedSAM model and the rendered mask with the initialized pose.
    Due to the limited space, we only visualize 4 images in each scene, although the total number of images is more than this number.
    }
    \label{fig:autoinit_4x4}
\end{figure}
